# Supplementary material for: Adaptive incentive for cross-silo federated learning: A multi-agent reinforcement learning approach
Source: arXiv:2302.07493 source file (2023-02-15)
Supplement: Supplementary file 1 [file appendix.tex]

\section{Appendix}\label{sec:appendix}

% \begin{spacing}{0.95}
% \emph{Proof of Theorem 1}. We need to prove that if the potential function given in Eq. (\ref{eq:thereoum1}) satisfies Eq. (\ref{eq:potential_function}). Here, we omit the superscript $[t]$ for concision. Let the decision of any $o_n$ change from $d_n$ to $d^{\prime}_{n}$, then, we have 
% \end{spacing}
% \begin{small}
% \vspace{-10pt}
% \begin{equation}\label{eq:U_prime}
%         \begin{aligned}
%     &\boldsymbol{U}({d}^{\prime}_{i},\boldsymbol{d}_{-i})
%         =\bm{P}\left(d^{\prime}_{i},\boldsymbol{d}_{-i}\right)-\sum_{j\in\mathcal{N}, j\neq i}\frac{ v_j d_{j}|\mathcal{D}_{n}|+C_{j}}{p_j}\\
%         &-\frac{ v_n d_{n}|\mathcal{D}_{n}|+C_{n}}{p_n}+\sum_{j\in \mathcal{N}}\frac{r_{n,j}(d^{\prime}_{n},d_j)}{p_n} +\sum_{j\in\mathcal{N}, j\neq i}\sum_{k\in \mathcal{N}}\frac{r_{j,k}(\pi_j,\pi_k)}{p_n}.\\
%     \end{aligned}
% \end{equation}
% \end{small}
% \noindent Subtracting Eq. (\ref{eq:U_prime}) from Eq. (\ref{eq:thereoum1}), we obtain
% \begin{small}
% \begin{equation}\label{eq:proof_theoreum1}
%  \begin{aligned}
%      p_n \left[ \boldsymbol{U}(d_n,\boldsymbol{d}_{-n}) - \boldsymbol{U}(d^{\prime}_{n},\boldsymbol{d}_{-n}) \right] =  
%     \boldsymbol{u}_{n}(d_n,\boldsymbol{d}_{-n}) - \boldsymbol{u}_{n}(d^{\prime}_{n},\boldsymbol{d}_{-n}),
%   \end{aligned}
% \end{equation}  
% which completes the proof.
% \end{small}$\qedsymbol$

\begin{spacing}{0.95}
\emph{The detailed derivation of policy gradient with function approximation in Eq. (\ref{eq:actor_optimization})}. By definition, $V^\pi(s)=\sum_d \pi(s,  d) Q^\pi(s,  d)$, we have 
% Therefore, the derivation writes as
% Here, we omit the subscript $n$ and replace $Q^\pi(s,  d)$ with $Q^\pi$  for concision. By definition, $V^\pi(s)=\sum_d \pi(s,  d) Q^\pi(s,  d)$
\end{spacing}
\begin{small}
\vspace{-7pt}
\begin{equation}
    \begin{aligned}
&\frac{\partial V^\pi(s)}{\partial \theta} =
% \frac{\partial}{\partial \theta} \sum_x \pi(s,  d) Q^\pi(s,  d) \\
\sum_d\left[\frac{\partial \pi(s,  d)}{\partial \theta} Q^\pi(s,  d)+\pi(s,  d) \frac{\partial}{\partial \theta} Q^\pi(s,  d)\right] \\
% &=\sum_d\Bigg[\frac{\partial \pi(s,  d)}{\partial \theta} Q^\pi(s,  d)+\pi(s,  d) \frac{\partial}{\partial \theta}\bigg[r(s,  d)\\ &+\sum_{s^{\prime}} \gamma P_n\left(s, s^{\prime}, d\right) V^\pi\left(s^{\prime}\right)\bigg]\Bigg] \\
&=\sum_d\left[\frac{\partial \pi(s,  d)}{\partial \theta} Q^\pi(s,  d)+\pi(s,  d) \sum_{s^{\prime}} \gamma P_r\left(s, s^{\prime}, d\right) \frac{\partial}{\partial \theta} V^\pi\left(s^{\prime}\right)\right] \\
&=\sum_{t=0}^{\infty} \sum_{s^{\prime}} \gamma^t \operatorname{Pr}\left(s ,s^{\prime}, t, \pi\right) \sum_d \frac{\partial \pi\left(s^{\prime}, d\right)}{\partial \theta} Q^\pi\left(s^{\prime}, d\right) \\
&=\sum_{s^{\prime} \in S} \sum_{t=0}^{\infty} \gamma^t \operatorname{Pr}\left(s , s^{\prime}, t, \pi\right) \sum_d \pi\left(s^{\prime}, d\right) \frac{\partial \log \pi\left(s^{\prime}, d\right)}{\partial \theta} Q^\pi\left(s^{\prime}, d\right) \\
&=\sum_{s^{\prime} \in \mathcal{S}} d^\pi\left(s^{\prime}\right) \sum_d \pi\left(s^{\prime}, d\right) \frac{\partial \log \pi\left(s^{\prime}, d\right)}{\partial \theta} Q^\pi\left(s^{\prime}, d\right),
\end{aligned}
\end{equation}
\end{small}%
\vspace{-5pt}
\begin{spacing}{0.95}
\noindent where $\operatorname{Pr}\left(s , s^{\prime}, t, \pi\right)$ indicates the probability of starting from state $s$ and ending with state $s^{\prime}$ within $t$ steps under policy $\pi$. Thus, we have
\end{spacing}
\vspace{-5pt}
\begin{small}
\begin{equation}
    \nabla_\theta V^\pi(s)=\sum_{s \in \mathcal{S}} d^\pi(s) \sum_d \pi(s,  d) \nabla_\theta \log \pi(s,  d) Q^\pi(s,  d),
\end{equation}
\end{small}%
\begin{spacing}{0.95}%
\noindent where $d^\pi(s)=\sum_{t=0}^{\infty} \gamma^t \operatorname{Pr}\left(s_0 , s, t, \pi\right)$ is the discounted state distribution.
% To be strict, it is not a standard distribution, since
% $$
% \sum_{s \in \mathcal{S}} d^\pi(s)=\sum_{s \in \mathcal{S}} \sum_{t=0}^{\infty} \gamma^t \operatorname{Pr}\left(s_0 , s_{:} k, \pi\right)=\sum_{t=0}^{\infty} \gamma^t \sum_{s \in S} \operatorname{Pr}\left(s_0 , s, k, \pi\right)=\sum_{t=0}^{\infty} \gamma^t=\frac{1}{1-\gamma} .
% $$
Therefore, when we take the expectation over the state $s \sim(1-\gamma) d^\pi$ and the action $d \sim \pi(s,  d)$, we have
\end{spacing}
\vspace{-5pt}
\vspace{-5pt}
\vspace{-5pt}
\begin{small}
\begin{equation}
    \begin{aligned}
\nabla_\theta V^\pi(s) &=\frac{1}{1-\gamma} \sum_{s \in \mathcal{S}}(1-\gamma) d^\pi \sum_s \pi(s,  d) \nabla_\theta \log \pi(s,  d) Q^\pi(s,  d) \\
&=\frac{1}{1-\gamma} \mathbb{E}_{\pi(\theta)}\left[\nabla_0 \log \pi(s,  d) Q^\pi(s,  d)\right] .
\end{aligned}
\end{equation}
\end{small}%
% In experinnents, we only care about the direction of the gradient, thus we usually omit the constant term $\frac{1}{(1-r)}$.
Since the observation $o$ which reflects the hidden state $s$ is sampled from the observation distribution $\rho^1(o)$. we know that
\begin{small}
\begin{equation}
    \begin{aligned}
\nabla_\theta L=\mathbb{E}^{[}\left[V^{\pi_\theta}(o) \mid \rho\right]=\mathbb{E}_{\pi_{\hat{n}}, \rho^1(o)}\left[\nabla_\theta \log \pi_\theta(o, d) Q^{\pi_\theta}(o, d)\right],
\end{aligned}
\end{equation}
\end{small}%
which confirms Eq. (\ref{eq:actor_optimization}).
